# Supplementary material for: TerrainMesh: Metric-Semantic Terrain Reconstruction from Aerial Images Using Joint 2D-3D Learning
Source: arXiv:2204.10993 source file (2024-01-16)
Supplement: Supplementary file 1 [file Appendix.tex]

\section{Appendix}
\label{sec:appendix}

Dear Editor-in-Chief,

We are submitting a paper, titled "TerrainMesh: Metric-Semantic Terrain Reconstruction from Aerial Images Using Joint 2D-3D Learning", to be considered for publication in the IEEE Transactions on Robotics. 
The paper considers the problem of metric-semantic mesh reconstruction of outdoor terrain using aerial RGB images. It can be combined with the popular feature-based keyframe SLAM to build dense metric-semantic model which can enable more complicated task like semantic exploration and navigation.

A preliminary version of the paper appeared at the 2021 IEEE International Conference on Robotics and Automation (ICRA). It included the problem formulation, theoretical development, and evaluation for geometric-only mesh reconstruction. This version improves the theoretical development and extends the approach to provide metric-semantic meshes. In this version, we introduce both mesh vertex spatial coordinates and semantic features and perform the mesh initialization and refinement stages using 2D feature extraction and 3D graph convolution. The new method can recover not only the height but also the semantic information on the mesh model. We evaluate our method on a new aerial image dataset with sparse depth measurements and ground-truth depth and semantic labels. We believe that our metric-semantic mesh reconstruction approach will enable feature-based SLAM algorithms to generate meaningful dense 3D model in real time, with key applications in environmental monitoring and security and surveillance. 

This is the first time that we submit a journal version of the paper, and the IEEE Transactions on Robotics is the only journal that we are submitting the manuscript to.

Thank you for considering our paper.

Best regards,

Qiaojun Feng and Nikolay Atanasov
